# Supplementary material for: Low-order Scaling $G_0W_0$ by Pair Atomic Density Fitting
Source: arXiv:2007.01581 source file (2020-11-12)
Supplement: Supplementary file 1 [file SI.pdf]

# Supporting Information for: Low-Order Scaling $G_0W_0$ by Pair Atomic Density Fitting

Arno Förster* and Lucas Visscher

*Theoretical Chemistry, Vrije Universiteit, De Boelelaan 1083, NL-1081 HV, Amsterdam, The Netherlands*

E-mail: a.t.l.foerster@vu.nl

## Contents

**List of Figures** **S1**

**List of Tables** **S1**

**S1 Additional figures** **S2**

**S2 Thresholds** **S2**

**S3 GW100 QP Energies** **S4**

**S4 GW5000 QP Energies** **S10**

**S5 Numerical frequency integration** **S16**

**References** **S17**

# List of Figures


S1 Errors for the HOMO-LUMO QP gap on the $G_0W_0$@PBE level of theory . . S2


# List of Tables


S1 Thresholds controlling distance effects in the PADF-$G_0W_0$ algorithm. All values are in Bohr. . . . . . . . . . . . . . . . . . . . . . . . . . . . . . . . S3

S2 $G_0W_0$@PBE HOMO QP energies for the GW100 database . . . . . . . . . . S4

S3 $G_0W_0$@PBE LUMO QP energies for the GW100 database . . . . . . . . . . S6

S4 $G_0W_0$@PBE0 HOMO and LUMO QP energies for the GW100 database . . . S8

S5 $G_0W_0$@PBE0 HOMO QP energies for 20 large systems from GW5000 . . . . S10

S6 $G_0W_0$@PBE0 LUMO QP energies for 20 large systems from GW5000 . . . . S11

S7 $G_0W_0$@PBE0 HOMO and LUMO QP energies for 250 randomly selected systems from GW5000 . . . . . . . . . . . . . . . . . . . . . . . . . . . . . . . . S12

S8 Parameters of the linear fits $f(x) = a \times x + b$ . . . . . . . . . . . . . . . . . . S16

# S1 Additional figures

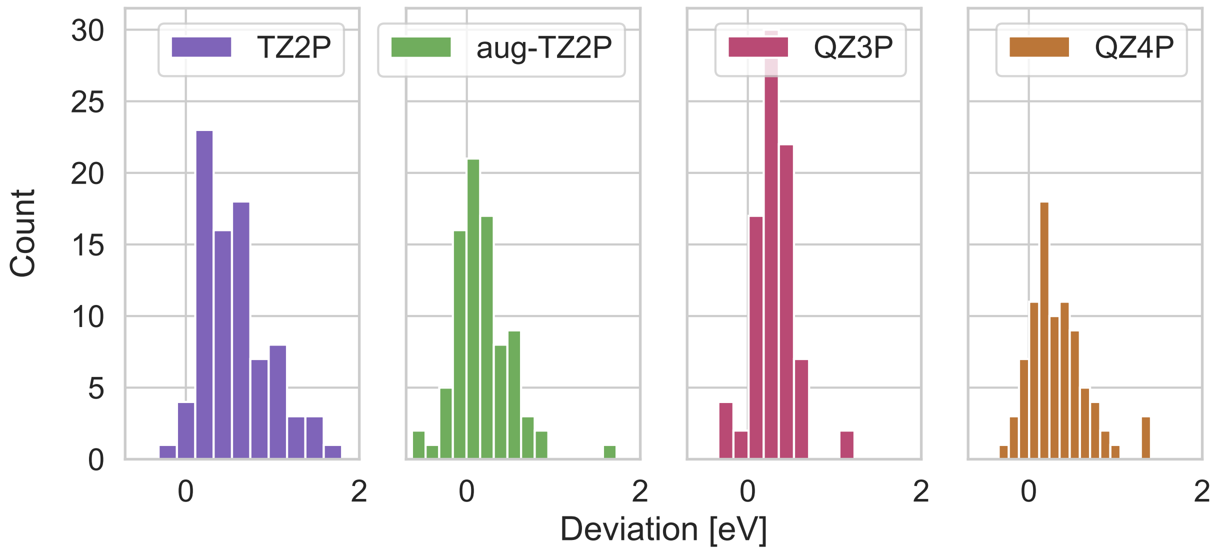


Figure S1: Distribution of errors for the HOMO-LUMO QP gap on the $G_0W_0$@PBE level of theory using four different STO-type basis sets. The error is in eV and with respect to the reference by Chelikowsky and coworkers.[1]

# S2 Thresholds

Beside from PADF, we employ further local approximations to reduce the asymptotic scaling of our algorithm from cubic to quadratic. For more details we refer to our recent work describing our MP2 implementation.[2]

A basis function is considered negligible for $|\boldsymbol{r}| > d_\mu$ if

$$|\chi_\mu(\boldsymbol{r})| < \epsilon_{bas} \quad \forall \, |\boldsymbol{r}| > d_\mu \ , \tag{1}$$

which implies that $C^{ABB}_{\mu\nu\beta} = C^{BAA}_{\nu\mu\alpha} = 0$ whenever

$$|\boldsymbol{R}_A - \boldsymbol{R}_B| > d_\mu + d_\nu \ , \tag{2}$$

and $\epsilon_{bas}$ is some (small) positive real number. In the same way, the interaction between two pair densities $\chi_\mu\chi_\nu$, $\chi_\kappa\chi_\lambda$ is evaluated via multipole expansion[3] (recall, that the fit functions

are always assumed to be centered on the second atom of the pair) if

$$|\boldsymbol{R}_B - \boldsymbol{R}_D| < d_\beta + d_\delta \quad \forall \beta, \delta \ , \tag{3}$$

where $d$ is defined by

$$|f_\beta(\boldsymbol{r})| < \epsilon_{multi} \quad \forall \ |\boldsymbol{r}| > d_\beta \ . \tag{4}$$

This is graphically illustrated in figure 1 in reference 2 (where we denoted $\epsilon_{bas}$ by $\vartheta_{DCAB}$, the procedure for $\epsilon_{multi}$ is the same).

Finally, when the Coulomb potential due to atom $A$, $V_c^A(\boldsymbol{r})$, does not overlap with any basis function on atom $B$, i.e. whenever

$$|\boldsymbol{R}_A - \boldsymbol{R}_B| < d_C + d_\nu \quad \forall \nu \in B \ , \tag{5}$$

where $d_C$ denotes the distance for which

$$|V_C^A(\boldsymbol{r})| < \epsilon_C \quad \forall |\boldsymbol{r}| > d_C \ , \tag{6}$$

the two atoms are defined as non-interacting. The values for the three thresholds we used in this work for all $GW$-calculations are given in S1.

Table S1: Thresholds controlling distance effects in the PADF-$G_0W_0$ algorithm. All values are in Bohr.

| | *Basic* | *Normal* | *Good* |
|---|---|---|---|
| $\epsilon_{multi}$ | $1 \times 10^{-2}$ | $5 \times 10^{-3}$ | $1 \times 10^{-3}$ |
| $\epsilon_{bas}$ | $1 \times 10^{-3}$ | $3 \times 10^{-4}$ | $1 \times 10^{-4}$ |
| $\epsilon_C$ | $3 \times 10^{-2}$ | $1 \times 10^{-2}$ | $1 \times 10^{-3}$ |

## S3 GW100 QP Energies

All values are also available in .CVS format

Table S2: $G_0W_0$@PBE HOMO QP energies for the GW100 database (all values in eV).

| | Name | TZ2P | aug-TZ2P | QZ3P | QZ4P |
|---|---|---|---|---|---|
| 1 | Helium | −22.904 | −22.716 | −23.102 | −23.063 |
| 2 | Neon | −20.087 | −20.048 | −20.077 | −19.821 |
| 3 | Argon | −14.707 | −14.585 | −14.698 | −14.663 |
| 4 | Krypton | −13.113 | −12.990 | −13.171 | −13.483 |
| 5 | Xenon | −11.546 | −11.543 | −11.690 | −11.690 |
| 6 | Hydrogen | −15.490 | −15.731 | −15.812 | −15.732 |
| 7 | Lithium dimer | −4.763 | −4.839 | −4.814 | −4.921 |
| 8 | Sodium dimer | −4.634 | −4.676 | −4.769 | −4.783 |
| 9 | Sodium tetramer | −3.905 | −3.970 | −4.039 | −4.006 |
| 10 | Sodium hexamer | −3.992 | −4.057 | −4.160 | −4.149 |
| 11 | Potassium dimer | −3.795 | −3.812 | −3.807 | −4.029 |
| 12 | Rubidium dimer | −3.669 | −3.710 | −3.959 | −3.959 |
| 13 | Nitrogen | −14.521 | −14.293 | −14.536 | −14.682 |
| 14 | Phosphorus dimer | −9.785 | −9.783 | −9.877 | −9.818 |
| 15 | Arsenic dimer | −9.057 | −9.050 | −9.195 | −9.489 |
| 16 | Fluorine | −14.389 | −14.279 | −14.606 | −14.572 |
| 17 | Chlorine | −10.714 | −10.675 | −10.816 | −10.600 |
| 18 | Bromine | −9.882 | −9.769 | −9.811 | −10.089 |
| 19 | Iodine | −9.188 | −8.808 | −8.704 | −8.701 |
| 20 | Methane | −13.663 | −13.675 | −13.796 | −13.805 |
| 21 | Ethane | −12.146 | −12.161 | −12.237 | −12.285 |
| 22 | Propane | −11.576 | −11.608 | −11.672 | −11.696 |
| 23 | Butane | −11.279 | −11.319 | −11.368 | −11.398 |
| 24 | Ethylene | −10.034 | −10.013 | −10.232 | −10.190 |
| 25 | Acetylene | −10.733 | −10.774 | −10.790 | −10.882 |
| 26 | Tetracarbon | −10.352 | −10.500 | −10.591 | −10.633 |
| 27 | Cyclopropane | −10.312 | −10.301 | −10.392 | −10.401 |
| 28 | Benzene | −8.638 | −8.557 | −8.844 | −8.945 |
| 29 | Cyclooctatetraene | −7.792 | −7.836 | −7.890 | −8.016 |
| 30 | Cyclopentadiene | −8.089 | −8.042 | −8.193 | −8.312 |
| 31 | Vinyl fluoride | −9.715 | −9.899 | −9.957 | −10.058 |
| 32 | Vinyl chloride | −9.429 | −9.467 | −9.535 | −9.518 |
| 33 | Vinyl bromide | −9.158 | −9.098 | −9.349 | −9.238 |
| 34 | Vinyl iodide | −8.777 | −8.731 | −8.806 | −8.819 |
| 35 | Tetrafluoromethane | −14.731 | −14.573 | −14.946 | −14.989 |
| 36 | Tetrachloromethane | −10.639 | −10.558 | −10.681 | −10.706 |
| 37 | Tetrabromomethane | −9.592 | −9.722 | −9.738 | −9.971 |
| 38 | Tetraiodomethane | −8.604 | −8.462 | −8.649 | −8.666 |
| 39 | Silane | −12.071 | −12.101 | −12.222 | −12.164 |
| 40 | Germane | −11.796 | −11.864 | −11.853 | −11.975 |
| 41 | Disilane | −10.027 | −10.435 | −10.145 | −10.166 |
| 42 | Pentasilane | −8.730 | −8.708 | −8.750 | −8.821 |
| 43 | Lithium hydride | −6.984 | −6.767 | −6.846 | −6.980 |
| 44 | Potassium hydride | −4.641 | −4.658 | −5.175 | −5.530 |
| 45 | Borane | −12.654 | −12.682 | −12.753 | −12.766 |
| 46 | Diborane(6) | −11.643 | −11.653 | −11.720 | −11.759 |
| 47 | Amonia | −10.196 | −9.889 | −10.177 | −10.100 |
| 48 | Hydrazoic acid | −10.109 | −10.053 | −10.220 | −10.234 |
| 49 | Phosphine | −9.900 | −9.813 | −10.024 | −10.045 |
| 50 | Arsine | −9.821 | −9.851 | −9.917 | −10.204 |

Continued on next page

| | Name | TZ2P | aug-TZ2P | QZ3P | QZ4P |
|---|---|---|---|---|---|
| 51 | Hydrogen sulfide | −9.667 | −9.652 | −9.696 | −9.839 |
| 52 | Hydrogen fluoride | −14.883 | −15.061 | −15.023 | −14.848 |
| 53 | Hydrogen chloride | −11.925 | −11.777 | −11.957 | −11.879 |
| 54 | Lithium fluoride | −9.928 | −9.603 | −9.792 | −9.932 |
| 55 | Magnesium fluoride | −12.475 | −12.005 | −11.968 | −12.191 |
| 56 | Titanium tetrafluoride | −13.465 | −13.475 | −14.080 | −13.450 |
| 57 | Aluminum fluoride | −13.459 | −13.845 | −13.935 | −13.936 |
| 58 | Boron monofluoride | −10.269 | −10.213 | −10.247 | −10.405 |
| 59 | Sulfur tetrafluoride | −11.642 | −11.678 | −11.783 | −11.808 |
| 60 | Potassium bromide | −7.430 | −7.405 | −7.382 | −7.848 |
| 61 | Gallium monochloride | −9.295 | −9.269 | −9.324 | −9.460 |
| 62 | Sodium chloride | −8.664 | −7.984 | −8.118 | −8.340 |
| 63 | Magnesium chloride | −10.600 | −10.660 | −10.700 | −10.767 |
| 64 | Aluminum iodide | −9.056 | −8.957 | −9.061 | −9.060 |
| 65 | Boron nitride | −10.915 | −10.859 | −10.994 | −10.808 |
| 66 | Hydrogen cyanide | −12.920 | −12.913 | −13.023 | −12.964 |
| 67 | Phosphorus mononitride | −10.776 | −11.316 | −10.846 | −10.873 |
| 68 | Hydrazine | −9.182 | −8.950 | −9.133 | −9.092 |
| 69 | Formaldehyde | −9.974 | −9.973 | −10.129 | −10.203 |
| 70 | Methanol | −10.257 | −10.140 | −10.408 | −10.371 |
| 71 | Ethanol | −9.849 | −9.784 | −9.998 | −9.991 |
| 72 | Acetaldehyde | −9.159 | −9.200 | −9.398 | −9.406 |
| 73 | Ethoxy ethane | −8.949 | −9.021 | −9.136 | −9.198 |
| 74 | Formic acid | −10.318 | −10.408 | −10.440 | −10.465 |
| 75 | Hydrogen peroxide | −10.641 | −10.494 | −10.775 | −10.862 |
| 76 | Water | −11.774 | −10.973 | −11.815 | −11.685 |
| 77 | Carbon dioxide | −12.811 | −12.820 | −12.973 | −12.927 |
| 78 | Carbon disulfide | −9.344 | −9.368 | −9.456 | −9.450 |
| 79 | Carbon oxide sulfide | −10.529 | −10.544 | −10.614 | −10.583 |
| 80 | Carbon oxide selenide | −9.800 | −9.809 | −9.921 | −10.230 |
| 81 | Carbon monoxide | −13.328 | −13.286 | −13.308 | −13.374 |
| 82 | Ozone | −11.566 | −11.372 | −11.782 | −11.677 |
| 83 | Sulfur dioxide | −11.441 | −11.472 | −11.627 | −11.580 |
| 84 | Beryllium monoxide | −9.180 | −9.120 | −9.108 | −9.356 |
| 85 | Magnesium monoxide | −7.061 | −6.651 | −6.920 | −6.933 |
| 86 | Toluene | −8.285 | −8.237 | −8.466 | −8.552 |
| 87 | Ethylbenzene | −8.239 | −8.183 | −8.415 | −8.435 |
| 88 | Hexafluorobenzene | −9.192 | −9.143 | −9.277 | −9.414 |
| 89 | Phenol | −7.965 | −7.984 | −8.159 | −8.150 |
| 90 | Aniline | −7.425 | −7.336 | −7.497 | −7.561 |
| 91 | Pyridine | −8.774 | −8.801 | −9.064 | −9.016 |
| 92 | Guanine | −7.442 | −7.429 | −7.521 | −7.618 |
| 93 | Adenine | −7.640 | −7.720 | −7.783 | −7.919 |
| 94 | Cytosine | −7.952 | −8.079 | −8.071 | −8.295 |
| 95 | Thymine | −8.406 | −8.434 | −8.513 | −8.616 |
| 96 | Uracil | −8.746 | −9.042 | −9.140 | −9.227 |
| 97 | Urea | −8.716 | −9.017 | −9.006 | −9.149 |
| 98 | Silver dimer | −6.915 | −6.940 | −6.982 | −6.972 |
| 99 | Copper dimer | −7.621 | −7.407 | −7.356 | −7.815 |
| 100 | Copper cyanide | −9.812 | −9.606 | −9.563 | −9.867 |

Table S3: $G_0W_0$@PBE LUMO QP energies for the GW100 database (all values in eV).

| | Name | TZ2P | aug-TZ2P | QZ3P | QZ4P |
|---|---|---|---|---|---|
| 1 | Helium | 10.614 | 2.916 | 4.396 | 2.842 |
| 2 | Neon | 11.236 | 2.903 | 2.630 | 3.755 |
| 3 | Argon | 8.690 | 2.010 | 3.087 | 1.857 |
| 4 | Krypton | 7.593 | 1.648 | 1.386 | 1.433 |
| 5 | Xenon | 5.563 | 5.563 | 1.329 | 1.329 |
| 6 | Hydrogen | 3.389 | 2.035 | 2.229 | 2.797 |
| 7 | Lithium dimer | −0.280 | −0.316 | −0.376 | −0.357 |
| 8 | Sodium dimer | −0.319 | −0.343 | −0.564 | −0.413 |
| 9 | Sodium tetramer | −0.546 | −0.588 | −0.722 | −0.682 |
| 10 | Sodium hexamer | −0.520 | −0.733 | −0.778 | −0.689 |
| 11 | Potassium dimer | −0.379 | −0.365 | −0.463 | −0.526 |
| 12 | Rubidium dimer | −0.477 | −0.505 | −0.663 | −0.663 |
| 13 | Nitrogen | 3.134 | 2.786 | 2.758 | 2.681 |
| 14 | Phosphorus dimer | −0.142 | −0.290 | −0.386 | −0.406 |
| 15 | Arsenic dimer | −0.442 | −0.500 | −0.528 | −0.880 |
| 16 | Fluorine | 0.600 | 0.479 | 0.321 | 0.225 |
| 17 | Chlorine | −0.133 | −0.268 | −0.359 | −0.431 |
| 18 | Bromine | −0.793 | −0.866 | −0.928 | −1.060 |
| 19 | Iodine | −1.090 | −1.075 | −1.346 | −1.345 |
| 20 | Methane | 2.238 | 0.871 | 1.114 | 1.583 |
| 21 | Ethane | 2.169 | 0.859 | 1.084 | 1.480 |
| 22 | Propane | 2.095 | 0.789 | 1.011 | 1.421 |
| 23 | Butane | 2.082 | 0.704 | 0.970 | 1.373 |
| 24 | Ethylene | 2.470 | 2.194 | 2.360 | 2.084 |
| 25 | Acetylene | 3.317 | 2.871 | 3.195 | 2.912 |
| 26 | Tetracarbon | −2.098 | −2.206 | −2.255 | −2.332 |
| 27 | Cyclopropane | 2.327 | 0.847 | 1.131 | 1.557 |
| 28 | Benzene | 1.489 | 1.361 | 1.381 | 1.244 |
| 29 | Cyclooctatetraene | 0.514 | 0.412 | 0.352 | 0.220 |
| 30 | Cyclopentadiene | 1.454 | 1.313 | 1.329 | 1.198 |
| 31 | Vinyl fluoride | 2.601 | 2.304 | 2.474 | 2.204 |
| 32 | Vinyl chloride | 1.935 | 1.693 | 1.763 | 1.615 |
| 33 | Vinyl bromide | 1.757 | 1.552 | 1.623 | 1.588 |
| 34 | Vinyl iodide | 1.359 | 1.243 | 1.068 | 0.938 |
| 35 | Tetrafluoromethane | 2.362 | 1.363 | 0.988 | 2.584 |
| 36 | Tetrachloromethane | 0.650 | 0.457 | 0.373 | 0.322 |
| 37 | Tetrabromomethane | −0.479 | −0.574 | −0.694 | −0.672 |
| 38 | Tetraiodomethane | −2.167 | −1.680 | −1.674 | −1.691 |
| 39 | Silane | 1.856 | 0.945 | 1.084 | 1.148 |
| 40 | Germane | 1.669 | 1.000 | 1.185 | 1.160 |
| 41 | Disilane | 2.048 | 0.918 | 1.807 | 1.620 |
| 42 | Pentasilane | 0.601 | 0.262 | 0.338 | 0.168 |
| 43 | Lithium hydride | 0.102 | 0.036 | 0.033 | 0.018 |
| 44 | Potassium hydride | 0.037 | −0.018 | −0.067 | −0.082 |
| 45 | Borane | 0.633 | 0.554 | 0.504 | 0.428 |
| 46 | Diborane(6) | 1.248 | 1.157 | 1.118 | 1.026 |
| 47 | Amonia | 1.933 | 0.907 | 1.105 | 1.044 |
| 48 | Hydrazoic acid | 2.051 | 1.791 | 1.778 | 1.678 |
| 49 | Phosphine | 1.604 | 0.841 | 0.951 | 1.237 |
| 50 | Arsine | 1.571 | 0.854 | 1.006 | 1.133 |
| 51 | Hydrogen sulfide | 1.701 | 0.955 | 1.017 | 1.014 |
| 52 | Hydrogen fluoride | 2.010 | 1.264 | 1.291 | 1.553 |
| 53 | Hydrogen chloride | 1.979 | 1.397 | 1.397 | 1.486 |
| 54 | Lithium fluoride | 0.131 | 0.088 | 0.100 | 0.079 |
| 55 | Magnesium fluoride | 0.089 | 0.001 | −0.015 | −0.064 |

Continued on next page

| | Name | TZ2P | aug-TZ2P | QZ3P | QZ4P |
|---|---|---|---|---|---|
| 56 | Titanium tetrafluoride | 0.961 | 0.941 | 0.887 | 0.595 |
| 57 | Aluminum fluoride | 0.636 | 0.318 | 0.265 | 0.068 |
| 58 | Boron monofluoride | 1.831 | 1.624 | 1.591 | 1.502 |
| 59 | Sulfur tetrafluoride | 1.121 | 0.879 | 0.795 | 0.458 |
| 60 | Potassium bromide | −0.197 | −0.208 | −0.232 | −0.229 |
| 61 | Gallium monochloride | 0.333 | 0.262 | 0.260 | 0.168 |
| 62 | Sodium chloride | −0.228 | −0.247 | −0.257 | −0.283 |
| 63 | Magnesium chloride | −0.141 | −0.184 | −0.242 | −0.304 |
| 64 | Aluminum iodide | −0.345 | −0.248 | −0.402 | −0.429 |
| 65 | Boron nitride | −2.942 | −3.006 | −3.128 | −3.172 |
| 66 | Hydrogen cyanide | 3.069 | 2.687 | 2.909 | 2.689 |
| 67 | Phosphorus mononitride | 0.481 | 0.259 | 0.188 | 0.137 |
| 68 | Hydrazine | 1.741 | 0.819 | 0.967 | 1.126 |
| 69 | Formaldehyde | 1.661 | 1.473 | 1.486 | 1.345 |
| 70 | Methanol | 2.090 | 1.025 | 1.188 | 1.446 |
| 71 | Ethanol | 1.981 | 0.936 | 1.097 | 1.380 |
| 72 | Acetaldehyde | 1.751 | 1.569 | 1.567 | 1.438 |
| 73 | Ethoxy ethane | 2.054 | 0.715 | 0.945 | 1.329 |
| 74 | Formic acid | 2.501 | 2.267 | 2.304 | 2.147 |
| 75 | Hydrogen peroxide | 2.962 | 2.558 | 2.613 | 2.390 |
| 76 | Water | 1.844 | 1.034 | 1.209 | 1.246 |
| 77 | Carbon dioxide | 4.169 | 1.286 | 1.629 | 1.114 |
| 78 | Carbon disulfide | 0.415 | 0.245 | 0.183 | 0.140 |
| 79 | Carbon oxide sulfide | 1.879 | 1.645 | 1.586 | 1.516 |
| 80 | Carbon oxide selenide | 1.495 | 1.360 | 1.299 | 1.283 |
| 81 | Carbon monoxide | 1.499 | 1.301 | 1.221 | 1.138 |
| 82 | Ozone | −1.246 | −1.445 | −1.590 | −1.671 |
| 83 | Sulfur dioxide | −0.203 | −0.409 | −0.502 | −0.575 |
| 84 | Beryllium monoxide | −1.711 | −1.777 | −1.733 | −1.878 |
| 85 | Magnesium monoxide | −1.321 | −1.435 | −1.500 | −1.539 |
| 86 | Toluene | 1.429 | 1.283 | 1.286 | 1.081 |
| 87 | Ethylbenzene | 1.467 | 1.311 | 1.309 | 1.121 |
| 88 | Hexafluorobenzene | 1.028 | 0.526 | 0.434 | 0.203 |
| 89 | Phenol | 1.429 | 1.280 | 1.293 | 1.161 |
| 90 | Aniline | 1.565 | 1.399 | 1.408 | 1.232 |
| 91 | Pyridine | 0.988 | 0.852 | 0.858 | 0.437 |
| 92 | Guanine | 1.196 | 0.992 | 0.913 | 0.801 |
| 93 | Adenine | 0.878 | 0.750 | 0.755 | 0.585 |
| 94 | Cytosine | 0.771 | 0.636 | 0.637 | 0.177 |
| 95 | Thymine | 0.602 | 0.460 | 0.438 | −0.030 |
| 96 | Uracil | 0.562 | 0.431 | 0.414 | 0.034 |
| 97 | Urea | 1.443 | 0.620 | 0.745 | 0.901 |
| 98 | Silver dimer | −0.669 | −0.673 | −0.762 | −0.760 |
| 99 | Copper dimer | −0.638 | −0.657 | −0.702 | −0.961 |
| 100 | Copper cyanide | −1.026 | −1.088 | −1.114 | −1.181 |

Table S4: $G_0W_0$@PBE0 HOMO and LUMO QP energies for the GW100 database (all values in eV).

| | | HOMO | | LUMO | |
|---|---|---|---|---|---|
| | Name | TZ2P | QZ4P | TZ2P | QZ4P |
| 1 | Helium | −23.202 | −23.546 | 10.677 | 2.813 |
| 2 | Neon | −20.402 | −20.381 | 11.331 | 3.794 |
| 3 | Argon | −14.989 | −14.933 | 8.743 | 1.879 |
| 4 | Krypton | −13.297 | −13.474 | 7.653 | 1.447 |
| 5 | Xenon | −11.761 | −11.935 | 5.598 | 1.349 |
| 6 | Hydrogen | −16.004 | −16.099 | 3.282 | 2.658 |
| 7 | Lithium dimer | −5.053 | −5.182 | −0.244 | −0.314 |
| 8 | Sodium dimer | −4.788 | −4.931 | −0.285 | −0.378 |
| 9 | Sodium tetramer | −4.058 | −4.186 | −0.515 | −0.645 |
| 10 | Sodium hexamer | −4.179 | −4.348 | −0.489 | −0.666 |
| 11 | Potassium dimer | −3.910 | −4.105 | −0.357 | −0.496 |
| 12 | Rubidium dimer | −3.808 | −4.335 | −0.384 | −0.564 |
| 13 | Nitrogen | −15.084 | −15.071 | 3.093 | 2.661 |
| 14 | Phosphorus dimer | −10.026 | −10.095 | −0.139 | −0.381 |
| 15 | Arsenic dimer | −9.238 | −9.657 | −0.440 | −0.630 |
| 16 | Fluorine | −14.899 | −15.140 | 0.626 | 0.298 |
| 17 | Chlorine | −10.995 | −11.120 | −0.083 | −0.368 |
| 18 | Bromine | −10.107 | −10.290 | −0.739 | −1.002 |
| 19 | Iodine | −9.131 | −9.237 | −1.103 | −1.269 |
| 20 | Methane | −14.044 | −14.138 | 2.266 | 1.564 |
| 21 | Ethane | −12.465 | −12.574 | 2.216 | 1.476 |
| 22 | Propane | −11.908 | −12.012 | 2.163 | 1.430 |
| 23 | Butane | −11.607 | −11.724 | 2.162 | 1.387 |
| 24 | Ethylene | −10.253 | −10.325 | 2.532 | 2.208 |
| 25 | Acetylene | −11.023 | −11.112 | 3.408 | 2.977 |
| 26 | Tetracarbon | −10.864 | −11.014 | −2.130 | −2.347 |
| 27 | Cyclopropane | −10.586 | −10.694 | 2.373 | 1.537 |
| 28 | Benzene | −8.933 | −9.184 | 1.682 | 1.356 |
| 29 | Cyclooctatetraene | −8.043 | −8.223 | 0.666 | 0.430 |
| 30 | Cyclopentadiene | −8.311 | −8.454 | 1.606 | 1.345 |
| 31 | Vinyl fluoride | −9.978 | −10.281 | 2.675 | 2.337 |
| 32 | Vinyl chloride | −9.709 | −9.833 | 2.001 | 1.688 |
| 33 | Vinyl bromide | −9.422 | −9.752 | 1.820 | 1.543 |
| 34 | Vinyl iodide | −8.831 | −9.128 | 1.435 | 1.094 |
| 35 | Tetrafluoromethane | −15.358 | −15.642 | 2.354 | 2.596 |
| 36 | Tetrachloromethane | −11.069 | −11.163 | 0.711 | 0.391 |
| 37 | Tetrabromomethane | −9.945 | −10.151 | −0.434 | −0.657 |
| 38 | Tetraiodomethane | −8.822 | −8.938 | −1.424 | −1.640 |
| 39 | Silane | −12.472 | −12.592 | 1.876 | 1.315 |
| 40 | Germane | −12.167 | −12.290 | 1.663 | 1.037 |
| 41 | Disilane | −10.343 | −10.467 | 1.630 | 1.048 |
| 42 | Pentasilane | −8.975 | −9.120 | 0.769 | 0.334 |
| 43 | Lithium hydride | −7.541 | −7.521 | 0.016 | −0.065 |
| 44 | Potassium hydride | −5.721 | −5.706 | −0.016 | −0.122 |
| 45 | Borane | −13.034 | −13.133 | 0.609 | 0.403 |
| 46 | Diborane(6) | −12.024 | −12.154 | 1.326 | 1.094 |
| 47 | Amonia | −10.520 | −10.486 | 1.923 | 1.309 |
| 48 | Hydrazoic acid | −10.439 | −10.573 | 2.006 | 1.625 |
| 49 | Phosphine | −10.163 | −10.321 | 1.609 | 1.223 |
| 50 | Arsine | −10.022 | −10.308 | 1.581 | 1.126 |
| 51 | Hydrogen sulfide | −9.916 | −10.012 | 1.671 | 1.128 |
| 52 | Hydrogen fluoride | −15.260 | −15.341 | 1.862 | 1.364 |

Continued on next page

| | | HOMO | | LUMO | |
|---|---|---|---|---|---|
| | Name | TZ2P | QZ4P | TZ2P | QZ4P |
| 53 | Hydrogen chloride | −12.137 | −12.104 | 1.816 | 1.342 |
| 54 | Lithium fluoride | −10.465 | −10.517 | −0.003 | −0.033 |
| 55 | Magnesium fluoride | −13.498 | −12.867 | 0.063 | −0.064 |
| 56 | Titanium tetrafluoride | −14.403 | −14.498 | 0.357 | 0.025 |
| 57 | Aluminum fluoride | −14.318 | −14.613 | 0.675 | 0.297 |
| 58 | Boron monofluoride | −10.663 | −10.727 | 1.738 | 1.402 |
| 59 | Sulfur tetrafluoride | −12.055 | −12.278 | 1.124 | 0.734 |
| 60 | Potassium bromide | −7.701 | −7.738 | −0.304 | −0.355 |
| 61 | Gallium monochloride | −9.472 | −9.633 | 0.284 | 0.137 |
| 62 | Sodium chloride | −8.495 | −8.655 | −0.337 | −0.390 |
| 63 | Magnesium chloride | −11.062 | −11.265 | −0.155 | −0.311 |
| 64 | Aluminum iodide | −9.300 | −9.427 | −0.200 | −0.384 |
| 65 | Boron nitride | −11.252 | −11.387 | −3.106 | −3.269 |
| 66 | Hydrogen cyanide | −13.248 | −13.330 | 3.078 | 2.656 |
| 67 | Phosphorus mononitride | −11.301 | −11.458 | 0.452 | 0.127 |
| 68 | Hydrazine | −9.459 | −9.493 | 1.746 | 1.082 |
| 69 | Formaldehyde | −10.399 | −10.614 | 1.677 | 1.357 |
| 70 | Methanol | −10.652 | −10.790 | 2.066 | 1.356 |
| 71 | Ethanol | −10.309 | −10.434 | 1.995 | 1.326 |
| 72 | Acetaldehyde | −9.726 | −9.927 | 1.838 | 1.530 |
| 73 | Ethoxy ethane | −9.413 | −9.634 | 2.132 | 1.337 |
| 74 | Formic acid | −10.823 | −11.102 | 2.562 | 2.217 |
| 75 | Hydrogen peroxide | −11.070 | −11.238 | 2.784 | 2.246 |
| 76 | Water | −12.096 | −12.261 | 1.770 | 1.249 |
| 77 | Carbon dioxide | −13.216 | −13.429 | 4.248 | 1.448 |
| 78 | Carbon disulfide | −9.590 | −9.795 | 0.385 | 0.128 |
| 79 | Carbon oxide sulfide | −10.821 | −10.895 | 1.865 | 1.520 |
| 80 | Carbon oxide selenide | −10.055 | −10.397 | 1.466 | 1.198 |
| 81 | Carbon monoxide | −13.866 | −13.891 | 1.377 | 1.052 |
| 82 | Ozone | −12.089 | −12.478 | −1.349 | −1.726 |
| 83 | Sulfur dioxide | −11.855 | −12.049 | −0.234 | −0.573 |
| 84 | Beryllium monoxide | −9.355 | −9.465 | −1.842 | −1.990 |
| 85 | Magnesium monoxide | −7.153 | −7.206 | −1.337 | −1.544 |
| 86 | Toluene | −8.565 | −8.758 | 1.594 | 1.289 |
| 87 | Ethylbenzene | −8.506 | −8.677 | 1.707 | 1.307 |
| 88 | Hexafluorobenzene | −9.560 | −9.695 | 0.992 | 0.075 |
| 89 | Phenol | −8.185 | −8.489 | 1.539 | 1.261 |
| 90 | Aniline | −7.633 | −7.848 | 1.596 | 1.396 |
| 91 | Pyridine | −9.378 | −9.479 | 1.063 | 0.849 |
| 92 | Guanine | −7.736 | −7.913 | 1.247 | 0.806 |
| 93 | Adenine | −8.013 | −8.183 | 1.014 | 0.801 |
| 94 | Cytosine | −8.337 | −8.535 | 0.831 | 0.598 |
| 95 | Thymine | −8.757 | −8.946 | 0.683 | 0.418 |
| 96 | Uracil | −9.130 | −9.304 | 0.631 | 0.381 |
| 97 | Urea | −9.507 | −9.711 | 1.469 | 0.907 |
| 98 | Silver dimer | −6.867 | −7.013 | −0.486 | −0.663 |
| 99 | Copper dimer | −7.471 | −7.622 | −0.477 | −0.602 |
| 100 | Copper cyanide | −10.130 | −10.082 | −0.945 | −1.075 |

## S4 GW5000 QP Energies

All values are also available in .CVS format

Table S5: $G_0W_0$@PBE0 HOMO QP energies for 20 large from GW5000 (all values in eV). The numbers in the second column refer to the system numbers in the reference[4] and the ordering of systems is the same as in the main text.

| | | aug-DZP | | TZ2P | |
|---|---|---|---|---|---|
| | Name | | Basic | Normal | Good |
| 1 | 53699 | −5.839 | −5.725 | −5.790 | −5.796 |
| 2 | 47797 | −7.020 | −6.993 | −7.024 | −7.024 |
| 3 | 47126 | −6.861 | −6.905 | −6.914 | −6.901 |
| 4 | 50280 | −6.169 | −6.184 | −6.243 | −6.241 |
| 5 | 48940 | −7.316 | −7.358 | −7.378 | −7.351 |
| 6 | 46250 | −6.172 | −6.062 | −6.082 | −6.135 |
| 7 | 45406 | −6.522 | −6.623 | −6.599 | −6.607 |
| 8 | 48237 | −7.035 | −7.047 | −7.077 | −7.095 |
| 9 | 44870 | −8.035 | −8.084 | −8.084 | −8.083 |
| 10 | 51751 | −5.707 | −5.837 | −5.851 | −5.848 |
| 11 | 47842 | −6.579 | −6.765 | −6.767 | −6.767 |
| 12 | 48180 | −7.614 | −7.722 | −7.721 | −7.720 |
| 13 | 44586 | −6.048 | −6.069 | −6.073 | −6.136 |
| 14 | 47776 | −8.377 | −8.618 | −8.618 | −8.617 |
| 15 | 49155 | −6.374 | −6.574 | −6.569 | −6.594 |
| 16 | 48578 | −7.562 | −7.651 | −7.650 | −7.649 |
| 17 | 47017 | −7.252 | −7.229 | −7.152 | −7.144 |
| 18 | 47010 | −6.373 | −6.547 | −6.550 | −6.562 |
| 19 | 48008 | −7.186 | −7.263 | −7.252 | −7.250 |
| 20 | 47960 | −6.036 | −5.896 | −5.981 | −5.983 |

Table S6: $G_0W_0$@PBE0 LUMO QP energies for 20 large from GW5000 (all values in eV) for different threshold qualities (for TZ2P). The numbers in the second column refer to the system numbers in the reference[4] and the ordering of systems is the same as in the main text.

| | | aug-DZP | TZ2P | | |
|---|---|---|---|---|---|
| | Name | | Basic | Normal | Good |
| 1 | 53699 | −1.910 | −1.797 | −1.862 | −1.872 |
| 2 | 47797 | −0.493 | −0.370 | −0.379 | −0.379 |
| 3 | 47126 | −0.775 | −0.658 | −0.658 | −0.657 |
| 4 | 50280 | −0.804 | −0.793 | −0.795 | −0.795 |
| 5 | 48940 | −0.303 | −0.255 | −0.251 | −0.251 |
| 6 | 46250 | −0.691 | −0.837 | −0.640 | −0.673 |
| 7 | 45406 | −0.703 | −0.607 | −0.606 | −0.606 |
| 8 | 48237 | −0.057 | −0.292 | −0.153 | −0.163 |
| 9 | 44870 | 0.119 | 0.127 | 0.127 | 0.127 |
| 10 | 51751 | −0.189 | −0.215 | −0.144 | −0.136 |
| 11 | 47842 | 0.017 | −0.123 | −0.125 | −0.125 |
| 12 | 48180 | −0.191 | −0.133 | −0.138 | −0.138 |
| 13 | 44586 | −0.492 | −0.514 | −0.513 | −0.513 |
| 14 | 47776 | 0.180 | 0.117 | 0.116 | 0.116 |
| 15 | 49155 | −0.284 | −0.305 | −0.347 | −0.346 |
| 16 | 48578 | 0.287 | 0.269 | 0.269 | 0.269 |
| 17 | 47017 | −1.803 | −1.363 | −1.498 | −1.482 |
| 18 | 47010 | 0.271 | 0.171 | 0.183 | 0.184 |
| 19 | 48008 | −0.475 | −0.346 | −0.341 | −0.333 |
| 20 | 47960 | −1.149 | −1.127 | −1.084 | −1.077 |

Table S7: $G_0W_0$@PBE0 HOMO and LUMO QP energies for 250 randomly selected systems from GW5000 (all values in eV) for different threshold qualities (for TZ2P). The numbers in the second column refer to the system numbers in the reference[4] and the ordering of systems is the same as in the main text.

| | | HOMO | | LUMO | |
|---|---|---|---|---|---|
| | Name | aug-DZP | TZ2P | aug-DZP | TZ2P |
| 1 | 10214 | −9.861 | −10.006 | −1.834 | −1.944 |
| 2 | 11403 | −10.740 | −10.937 | 0.711 | 0.604 |
| 3 | 23303 | −7.077 | −7.261 | −1.066 | −1.232 |
| 4 | 37765 | −8.934 | −9.091 | 0.222 | 0.145 |
| 5 | 5760 | −10.026 | −10.543 | 0.145 | −0.020 |
| 6 | 18255 | −8.425 | −8.570 | −0.793 | −0.841 |
| 7 | 21895 | −8.903 | −9.097 | 0.201 | 0.121 |
| 8 | 15634 | −7.972 | −8.162 | 0.451 | 0.388 |
| 9 | 12569 | −9.043 | −9.146 | −0.011 | −0.100 |
| 10 | 27595 | −9.125 | −9.285 | −0.809 | −0.885 |
| 11 | 10450 | −7.374 | −7.564 | 0.094 | 0.037 |
| 12 | 56782 | −8.312 | −8.510 | 0.027 | −0.064 |
| 13 | 37128 | −8.136 | −8.348 | −1.662 | −1.838 |
| 14 | 25240 | −9.216 | −9.354 | 0.292 | 0.231 |
| 15 | 55516 | −8.685 | −8.858 | −0.031 | −0.089 |
| 16 | 54009 | −7.426 | −7.530 | 0.335 | 0.331 |
| 17 | 9202 | −7.869 | −8.073 | −0.653 | −0.806 |
| 18 | 22078 | −6.960 | −7.144 | −1.100 | −1.134 |
| 19 | 17502 | −8.115 | −8.266 | −0.226 | −0.302 |
| 20 | 1942 | −7.509 | −7.669 | 0.466 | 0.418 |
| 21 | 57610 | −7.689 | −7.844 | 0.398 | 0.374 |
| 22 | 2869 | −8.306 | −8.448 | −0.618 | −0.703 |
| 23 | 40494 | −7.665 | −7.827 | −0.224 | −0.289 |
| 24 | 60360 | −8.312 | −8.458 | −0.189 | −0.287 |
| 25 | 13505 | −7.319 | −7.417 | −0.067 | −0.098 |
| 26 | 59304 | −9.199 | −9.437 | −1.126 | −1.302 |
| 27 | 57383 | −8.917 | −9.130 | −0.710 | −0.862 |
| 28 | 55803 | −8.678 | −8.878 | −0.507 | −0.564 |
| 29 | 32571 | −8.680 | −8.879 | 0.200 | 0.181 |
| 30 | 4257 | −7.909 | −8.113 | 0.193 | 0.167 |
| 31 | 22407 | −8.448 | −8.592 | −1.023 | −1.093 |
| 32 | 33146 | −8.693 | −8.854 | 0.270 | 0.187 |
| 33 | 4465 | −7.682 | −7.779 | −0.226 | −0.252 |
| 34 | 3387 | −7.360 | −7.458 | −0.335 | −0.399 |
| 35 | 1761 | −7.816 | −7.961 | 0.120 | 0.041 |
| 36 | 7474 | −7.871 | −8.051 | −0.266 | −0.347 |
| 37 | 60545 | −7.566 | −7.687 | 0.031 | −0.023 |
| 38 | 56584 | −9.642 | −9.767 | −0.809 | −0.909 |
| 39 | 55110 | −8.095 | −8.217 | 0.282 | 0.221 |
| 40 | 53842 | −7.954 | −8.042 | −0.781 | −0.810 |
| 41 | 60749 | −7.468 | −7.619 | −0.637 | −0.687 |
| 42 | 58846 | −7.789 | −7.951 | 0.162 | 0.094 |
| 43 | 10698 | −9.038 | −9.184 | −0.435 | −0.456 |
| 44 | 389 | −8.086 | −8.201 | −0.178 | −0.158 |
| 45 | 55259 | −7.354 | −7.482 | −0.507 | −0.587 |
| 46 | 57147 | −6.917 | −7.026 | −0.214 | −0.289 |
| 47 | 6527 | −8.345 | −8.420 | −0.878 | −0.922 |
| 48 | 54908 | −6.809 | −6.990 | −1.443 | −1.525 |
| 49 | 6838 | −8.484 | −8.615 | 0.258 | 0.224 |
| 50 | 46362 | −8.312 | −8.474 | 0.350 | 0.277 |
| 51 | 48399 | −7.424 | −7.579 | −0.774 | −0.829 |
| 52 | 61346 | −7.545 | −7.685 | 0.158 | 0.123 |
| 53 | 2686 | −7.462 | −7.621 | −0.997 | −1.067 |

Continued on next page

| | | HOMO | | LUMO | |
|---|---|---|---|---|---|
| | Name | aug-DZP | TZ2P | aug-DZP | TZ2P |
| 54 | 60181 | −7.597 | −7.784 | −0.609 | −0.661 |
| 55 | 6247 | −7.542 | −7.673 | 0.220 | 0.160 |
| 56 | 38315 | −8.282 | −8.424 | −0.255 | −0.321 |
| 57 | 33531 | −7.203 | −7.369 | −0.156 | −0.210 |
| 58 | 16444 | −7.931 | −8.148 | −0.395 | −0.476 |
| 59 | 10978 | −6.983 | −7.113 | 0.222 | 0.178 |
| 60 | 59849 | −8.296 | −8.534 | 0.165 | 0.119 |
| 61 | 12919 | −7.256 | −7.435 | −0.022 | −0.086 |
| 62 | 48653 | −7.273 | −7.404 | −1.096 | −1.179 |
| 63 | 4002 | −7.708 | −7.870 | −1.808 | −1.902 |
| 64 | 31853 | −7.484 | −7.623 | −0.546 | −0.609 |
| 65 | 25789 | −8.381 | −8.506 | 0.068 | 0.030 |
| 66 | 13712 | −7.521 | −7.654 | −0.637 | −0.727 |
| 67 | 21105 | −7.866 | −8.009 | −1.764 | −1.860 |
| 68 | 40764 | −8.239 | −8.346 | −1.573 | −1.632 |
| 69 | 56219 | −8.425 | −8.592 | −0.437 | −0.493 |
| 70 | 56050 | −8.389 | −8.579 | 0.335 | 0.285 |
| 71 | 45218 | −7.913 | −7.973 | −0.105 | −0.165 |
| 72 | 23028 | −8.367 | −8.546 | −0.147 | −0.235 |
| 73 | 14226 | −7.317 | −7.483 | 0.199 | 0.143 |
| 74 | 7729 | −8.470 | −8.595 | −0.471 | −0.543 |
| 75 | 54412 | −8.211 | −8.433 | −0.651 | −0.749 |
| 76 | 59631 | −7.101 | −7.249 | −0.358 | −0.437 |
| 77 | 19910 | −9.251 | −9.407 | −0.854 | −0.920 |
| 78 | 15429 | −6.181 | −6.355 | −0.425 | −0.483 |
| 79 | 28162 | −6.974 | −7.206 | 0.151 | 0.079 |
| 80 | 8509 | −8.713 | −8.847 | 0.022 | −0.063 |
| 81 | 56406 | −7.024 | −7.174 | −0.334 | −0.387 |
| 82 | 54233 | −7.399 | −7.523 | 0.339 | 0.308 |
| 83 | 41377 | −7.968 | −8.135 | −0.020 | −0.068 |
| 84 | 23853 | −7.182 | −7.335 | 0.054 | −0.006 |
| 85 | 21611 | −6.323 | −6.450 | −0.365 | −0.393 |
| 86 | 60961 | −7.611 | −7.777 | −0.825 | −0.879 |
| 87 | 58206 | −6.707 | −6.803 | −0.498 | −0.536 |
| 88 | 24031 | −5.993 | −6.174 | 0.023 | −0.050 |
| 89 | 1627 | −7.198 | −7.367 | −1.077 | −1.217 |
| 90 | 16 | −6.928 | −7.094 | 0.337 | 0.296 |
| 91 | 584 | −10.062 | −10.224 | −1.184 | −1.295 |
| 92 | 39917 | −7.507 | −7.710 | 0.342 | 0.272 |
| 93 | 39685 | −7.540 | −7.712 | −0.573 | −0.672 |
| 94 | 26685 | −7.586 | −7.734 | −0.290 | −0.333 |
| 95 | 22875 | −7.158 | −7.342 | 0.311 | 0.254 |
| 96 | 964 | −7.808 | −8.013 | −0.114 | −0.168 |
| 97 | 58653 | −8.841 | −8.947 | 0.122 | 0.008 |
| 98 | 26821 | −7.647 | −7.835 | 0.000 | −0.028 |
| 99 | 18460 | −6.755 | −6.904 | −0.617 | −0.667 |
| 100 | 23652 | −7.581 | −7.792 | 0.102 | −0.071 |
| 101 | 25412 | −7.473 | −7.715 | −0.322 | −0.385 |
| 102 | 21210 | −7.677 | −7.848 | 0.030 | −0.036 |
| 103 | 25995 | −7.012 | −7.124 | 0.115 | 0.065 |
| 104 | 212 | −7.697 | −7.860 | −0.208 | −0.258 |
| 105 | 59124 | −6.851 | −7.021 | −0.616 | −1.054 |
| 106 | 27801 | −7.611 | −7.717 | 0.181 | 0.147 |
| 107 | 53566 | −9.270 | −9.509 | 0.679 | 0.587 |
| 108 | 45995 | −7.406 | −7.606 | −0.072 | −0.193 |
| 109 | 21361 | −8.067 | −8.185 | −1.063 | −1.117 |
| 110 | 1145 | −7.097 | −7.242 | −0.387 | −0.429 |
| 111 | 54680 | −6.957 | −7.115 | 0.197 | 0.092 |
| 112 | 28450 | −7.101 | −7.263 | −0.651 | −0.683 |

Continued on next page

| | | HOMO | | LUMO | |
|---|---|---|---|---|---|
| | Name | aug-DZP | TZ2P | aug-DZP | TZ2P |
| 113 | 16704 | −5.880 | −6.167 | −0.812 | −0.871 |
| 114 | 58443 | −8.475 | −8.668 | 0.447 | 0.347 |
| 115 | 3793 | −8.475 | −8.622 | 0.145 | 0.141 |
| 116 | 26458 | −7.307 | −7.474 | 0.183 | 0.120 |
| 117 | 20821 | −7.881 | −8.063 | −0.640 | −0.718 |
| 118 | 20649 | −7.447 | −7.584 | 0.390 | 0.314 |
| 119 | 57896 | −7.321 | −7.394 | −0.314 | −0.393 |
| 120 | 27000 | −7.278 | −7.337 | 0.126 | 0.094 |
| 121 | 24951 | −7.149 | −7.304 | −0.119 | −0.151 |
| 122 | 20065 | −7.660 | −7.808 | −0.355 | −0.427 |
| 123 | 35442 | −6.787 | −6.892 | −0.473 | −0.471 |
| 124 | 38639 | −6.204 | −6.352 | 0.059 | 0.011 |
| 125 | 24201 | −6.454 | −6.602 | 0.298 | 0.267 |
| 126 | 20311 | −8.335 | −8.508 | 0.270 | 0.260 |
| 127 | 19347 | −8.017 | −8.218 | −1.483 | −1.564 |
| 128 | 18611 | −8.179 | −8.375 | 0.477 | 0.361 |
| 129 | 1304 | −8.403 | −8.479 | −1.140 | −1.177 |
| 130 | 2403 | −6.949 | −7.035 | −0.448 | −0.522 |
| 131 | 19664 | −8.339 | −8.503 | −0.571 | −0.587 |
| 132 | 61133 | −7.001 | −7.153 | 0.033 | −0.037 |
| 133 | 48162 | −7.819 | −7.938 | −0.701 | −0.736 |
| 134 | 27374 | −7.595 | −7.741 | 0.223 | 0.194 |
| 135 | 18825 | −7.021 | −7.133 | −0.364 | −0.399 |
| 136 | 19062 | −7.293 | −7.461 | 0.202 | 0.105 |
| 137 | 47200 | −6.802 | −6.979 | −0.200 | −0.241 |
| 138 | 3133 | −10.356 | −10.544 | −1.231 | −1.354 |
| 139 | 26246 | −7.579 | −7.784 | −0.421 | −0.539 |
| 140 | 24722 | −6.758 | −7.044 | 0.280 | −0.011 |
| 141 | 24419 | −8.315 | −8.426 | 0.289 | 0.290 |
| 142 | 2142 | −7.871 | −7.985 | −0.430 | −0.475 |
| 143 | 1415 | −7.555 | −7.733 | 0.417 | 0.380 |
| 144 | 9040 | −6.694 | −6.832 | 0.309 | 0.297 |
| 145 | 30647 | −7.499 | −7.646 | 0.106 | 0.083 |
| 146 | 29484 | −7.657 | −7.799 | −0.237 | −0.308 |
| 147 | 28674 | −7.811 | −8.018 | 0.210 | 0.173 |
| 148 | 50401 | −7.342 | −7.635 | 0.310 | 0.225 |
| 149 | 16245 | −7.276 | −7.424 | 0.227 | 0.186 |
| 150 | 12004 | −7.049 | −7.356 | 0.035 | −0.078 |
| 151 | 14979 | −8.341 | −8.596 | 0.391 | 0.313 |
| 152 | 8314 | −8.666 | −8.817 | 0.430 | 0.390 |
| 153 | 13321 | −7.654 | −7.828 | −0.867 | −0.921 |
| 154 | 5330 | −8.041 | −8.212 | −0.128 | −0.205 |
| 155 | 30510 | −6.565 | −6.589 | −0.052 | −0.040 |
| 156 | 12143 | −8.016 | −8.180 | −0.353 | −0.437 |
| 157 | 7902 | −7.937 | −7.989 | −0.013 | 0.003 |
| 158 | 7348 | −7.844 | −8.021 | 0.265 | 0.265 |
| 159 | 4727 | −7.459 | −7.633 | 0.374 | 0.265 |
| 160 | 45485 | −7.783 | −7.883 | −1.034 | −1.066 |
| 161 | 30240 | −6.984 | −6.982 | 0.265 | 0.253 |
| 162 | 29288 | −8.967 | −9.193 | 0.278 | 0.183 |
| 163 | 5948 | −6.558 | −6.674 | 0.186 | 0.173 |
| 164 | 14670 | −7.744 | −7.898 | −0.385 | −0.381 |
| 165 | 12405 | −7.611 | −7.782 | 0.014 | −0.028 |
| 166 | 8115 | −7.624 | −7.807 | −0.420 | −0.444 |
| 167 | 22699 | −7.751 | −8.181 | −1.044 | −1.095 |
| 168 | 13736 | −6.935 | −7.027 | 0.028 | 0.046 |
| 169 | 9844 | −8.092 | −8.268 | 0.049 | 0.019 |
| 170 | 8740 | −7.723 | −7.841 | 0.073 | 0.101 |
| 171 | 46991 | −8.445 | −8.586 | −0.339 | −0.390 |

Continued on next page

| | | HOMO | | LUMO | |
|---|---|---|---|---|---|
| | Name | aug-DZP | TZ2P | aug-DZP | TZ2P |
| 172 | 30014 | −6.665 | −6.786 | −0.843 | −0.860 |
| 173 | 28006 | −7.303 | −7.427 | −0.231 | −0.235 |
| 174 | 16849 | −7.541 | −7.693 | 0.065 | 0.007 |
| 175 | 30833 | −7.397 | −7.517 | −0.540 | −0.616 |
| 176 | 13722 | −7.551 | −7.710 | −0.140 | −0.193 |
| 177 | 4986 | −8.325 | −8.469 | 0.196 | 0.276 |
| 178 | 31114 | −7.323 | −7.491 | −0.103 | −0.159 |
| 179 | 29738 | −7.666 | −7.778 | 0.292 | 0.275 |
| 180 | 15938 | −7.645 | −7.784 | 0.021 | 0.007 |
| 181 | 31332 | −7.543 | −7.686 | −0.123 | −0.166 |
| 182 | 9538 | −8.261 | −8.320 | −1.122 | −1.133 |
| 183 | 5179 | −7.012 | −7.116 | −0.740 | −0.738 |
| 184 | 28988 | −7.242 | −7.501 | 0.034 | −0.078 |
| 185 | 14098 | −6.731 | −6.865 | −0.217 | −0.263 |
| 186 | 52978 | −8.001 | −8.096 | 0.675 | 0.590 |
| 187 | 13151 | −7.525 | −7.712 | 0.208 | 0.137 |
| 188 | 35225 | −7.648 | −7.882 | 0.436 | 0.299 |
| 189 | 31529 | −7.470 | −7.636 | 0.327 | 0.301 |
| 190 | 13702 | −6.510 | −6.649 | 0.427 | 0.440 |
| 191 | 7071 | −7.105 | −7.254 | −0.017 | −0.075 |
| 192 | 47575 | −7.469 | −7.615 | −0.454 | −0.450 |
| 193 | 15273 | −7.085 | −7.261 | 0.163 | 0.086 |
| 194 | 13760 | −7.038 | −7.082 | −0.146 | −0.132 |
| 195 | 11661 | −8.027 | −8.226 | 0.330 | 0.283 |
| 196 | 11151 | −7.744 | −7.844 | −0.402 | −0.447 |
| 197 | 42090 | −7.331 | −7.487 | 0.026 | −0.040 |
| 198 | 38920 | −6.739 | −6.840 | −0.697 | −0.634 |
| 199 | 36205 | −8.119 | −8.277 | −0.583 | −0.622 |
| 200 | 32294 | −6.457 | −6.550 | −1.260 | −1.284 |
| 201 | 18111 | −6.820 | −6.925 | −0.024 | −0.063 |
| 202 | 42908 | −6.885 | −7.107 | −0.035 | −0.149 |
| 203 | 51981 | −8.108 | −8.233 | −0.143 | −0.135 |
| 204 | 40978 | −8.508 | −8.649 | 0.492 | 0.572 |
| 205 | 49946 | −7.363 | −7.598 | −0.086 | −0.164 |
| 206 | 44205 | −7.460 | −7.071 | −0.606 | −0.212 |
| 207 | 43090 | −6.498 | −6.596 | −0.758 | −0.787 |
| 208 | 40143 | −7.710 | −7.844 | −0.574 | −0.578 |
| 209 | 49106 | −7.441 | −7.580 | −0.552 | −0.572 |
| 210 | 34005 | −7.253 | −7.336 | −0.045 | −0.017 |
| 211 | 39175 | −6.431 | −6.552 | 0.057 | 0.040 |
| 212 | 36515 | −7.551 | −7.698 | −0.180 | −0.239 |
| 213 | 43905 | −7.235 | −7.392 | 0.080 | 0.039 |
| 214 | 34913 | −6.783 | −6.961 | −0.113 | −0.173 |
| 215 | 37381 | −7.796 | −8.050 | 0.459 | 0.359 |
| 216 | 51317 | −6.743 | −6.889 | −0.284 | −0.317 |
| 217 | 43385 | −7.059 | −7.233 | −0.349 | −0.393 |
| 218 | 42754 | −6.852 | −7.027 | −0.246 | −0.363 |
| 219 | 41897 | −7.510 | −7.653 | −0.400 | −0.616 |
| 220 | 39418 | −7.737 | −7.875 | −0.556 | −0.574 |
| 221 | 33692 | −8.145 | −8.312 | −0.282 | −0.331 |
| 222 | 53229 | −8.268 | −8.427 | −0.081 | −0.069 |
| 223 | 43634 | −7.465 | −7.643 | 0.016 | −0.114 |
| 224 | 41571 | −6.212 | −6.399 | −0.406 | −0.501 |
| 225 | 17264 | −7.013 | −7.084 | −0.680 | −0.698 |
| 226 | 42424 | −7.600 | −7.755 | 0.385 | 0.326 |
| 227 | 17807 | −7.216 | −7.358 | 0.146 | 0.103 |
| 228 | 35790 | −7.028 | −7.096 | −0.123 | −0.073 |
| 229 | 52590 | −6.456 | −6.417 | −0.433 | −0.611 |
| 230 | 36735 | −6.913 | −7.126 | −0.899 | −1.041 |

Continued on next page

| | | HOMO | | LUMO | |
|---|---|---|---|---|---|
| | Name | aug-DZP | TZ2P | aug-DZP | TZ2P |
| 231 | 34307 | −7.269 | −7.425 | −0.919 | −0.915 |
| 232 | 33372 | −7.157 | −7.421 | 0.383 | 0.239 |
| 233 | 32947 | −6.888 | −7.021 | −0.542 | −0.579 |
| 234 | 38018 | −6.897 | −7.060 | −0.063 | −0.079 |
| 235 | 34564 | −6.437 | −6.467 | −0.253 | −0.318 |
| 236 | 16982 | −7.388 | −7.630 | 0.032 | −0.058 |
| 237 | 51045 | −7.286 | −7.415 | 0.256 | 0.248 |
| 238 | 51639 | −7.426 | −7.573 | −0.803 | −0.879 |
| 239 | 48947 | −6.835 | −6.850 | 0.108 | 0.159 |
| 240 | 46610 | −8.042 | −8.316 | 0.220 | 0.066 |
| 241 | 45666 | −8.281 | −8.487 | 0.327 | 0.232 |
| 242 | 46821 | −6.772 | −6.926 | −0.570 | −0.621 |
| 243 | 52259 | −7.938 | −8.132 | −0.358 | −0.368 |
| 244 | 50771 | −7.554 | −7.693 | 0.115 | 0.153 |
| 245 | 49471 | −6.039 | −6.103 | −1.372 | −1.402 |
| 246 | 50224 | −8.174 | −8.341 | −0.239 | −0.231 |
| 247 | 47960 | −5.915 | −5.982 | −1.035 | −1.077 |
| 248 | 44870 | −7.972 | −8.083 | 0.128 | 0.127 |
| 249 | 44586 | −6.048 | −6.127 | −0.492 | −0.512 |
| 250 | 47797 | −6.961 | −7.024 | −0.445 | −0.379 |

Table S8: Parameters of the linear fits $f(x) = a \times x + b$ shown in figure 8 in the main text. All value are in eV.

| | HOMO | | LUMO | | gap | |
|---|---|---|---|---|---|---|
| basis set | a | b | a | b | a | b |
| aug-DZP | −0.000 431 | 0.653 289 | −0.000 734 | 0.814 004 | −0.000 303 | 0.160 719 |
| TZ2P | −0.000 285 | 0.482 206 | −0.000 524 | 0.731 793 | −0.000 239 | 0.249 591 |
| def-TZVP | −0.000 136 | 0.400 648 | −0.000 365 | 0.515 398 | −0.000 229 | 0.114 750 |
| def-QZVP | −0.000 126 | 0.190 429 | −0.000 247 | 0.245 059 | −0.000 121 | 0.054 630 |

# S5 Numerical frequency integration

All pretabulated grid points and integration weights (the latter are needed for RPA correlation energies) used in our work to obtain converged imaginary frequency grids are available as .txt-file. For all tabulated ranges, the file also includes the $L_2$-norm of the minimized error-distribution function[5] for all ranges of transition energies $[1, \epsilon_{max}/\epsilon_{min}]$, where $\epsilon_{min}$ ($\epsilon_{min}$) denotes the smallest (largest) KS orbital energy difference.

$$\|\eta(x;\{\gamma_i,\omega_i\})\|_2 = \left\| \frac{1}{x} - \frac{1}{\pi}\sum_{i=1}^{N_\omega} \gamma_i \left(\frac{2x}{x^2+\omega_i^2}\right)^2 \right\|_2 , \quad x \in [1, \epsilon_{max}/\epsilon_{min}] . \tag{7}$$

# References


(1) Gao, W.; Chelikowsky, J. R. Real-Space Based Benchmark of G0W0 Calculations on GW100: Effects of Semicore Orbitals and Orbital Reordering. *J. Chem. Theory Comput.* **2019**, *15*, 5299–5307.

(2) Förster, A.; Franchini, M.; van Lenthe, E.; Visscher, L. A Quadratic Pair Atomic Resolution of the Identity Based SOS-AO-MP2 Algorithm Using Slater Type Orbitals. *J. Chem. Theory Comput.* **2020**, *16*, 875–891.

(3) Jackson, J. D. *Classical electrodynamics*; AAPT, 1999.

(4) Stuke, A.; Kunkel, C.; Golze, D.; Todorović, M.; Margraf, J. T.; Reuter, K.; Rinke, P.; Oberhofer, H. Atomic structures and orbital energies of 61,489 crystal-forming organic molecules. *Sci. Data* **2020**, *7*, 1–11.

(5) Kaltak, M.; Klimeš, J.; Kresse, G. Low scaling algorithms for the random phase approximation: Imaginary time and laplace transformations. *J. Chem. Theory Comput.* **2014**, *10*, 2498–2507.
